# Supplementary material for: Can collaborative learning be private, robust and scalable?
Source: arXiv:2205.02652 source file (2022-08-08)
Supplement: Supplementary file 1 [file supplement_decaf_paper6.pdf]

# Can collaborative learning be private, robust and scalable?

Dmitrii Usynin[1,2,3], Helena Klause[1], Johannes Paetzold[1], Daniel Rueckert[1,2,3], and Georgios Kaissis[1,2]

[1] Artificial Intelligence in Medicine and Healthcare, Technical University of Munich, Munich, Germany
[2] Institute of Diagnostic and Interventional Radiology, Technical University of Munich, Munich, Germany
[3] Department of Computing, Imperial College London, London, United Kingdom

## 1 Supplementary Material

### 1.1 Threat model

Our threat model includes two settings. The first one is an active train-time, WB attacker, who is *malicious* (actively intervenes in the training process). The second type is an active inference-time attacker with a partial WB model access (WB access to a model similar to the one being attacked).

### 1.2 Performance of the original models

| | CIFAR-10 | PPPD |
|---|---|---|
| ResNet-9 | 81.8% | 87.9% |
| ResNet-18 | 73.2% | 93.2% |

**Table 1.** Classification accuracy (non-private)

| | CIFAR-10 | PPPD |
|---|---|---|
| ResNet-9 | 52.3% | 70.3% |
| ResNet-18 | 44.4% | 67.1% |

**Table 2.** Classification accuracy ($\varepsilon = 1.7$)

| | CIFAR-10 | PPPD |
|---|---|---|
| ResNet-9 | 57.5% | 73.6% |
| ResNet-18 | 47.3% | 67.9% |

**Table 3.** Classification accuracy ($\varepsilon = 3.4$)

| | CIFAR-10 | PPPD |
|---|---|---|
| ResNet-9 | 59.5% | 75.1% |
| ResNet-18 | 54.9% | 68.6% |

**Table 4.** Classification accuracy ($\varepsilon = 7.0$)

### 1.3 Adversarial training results for different privacy regimes

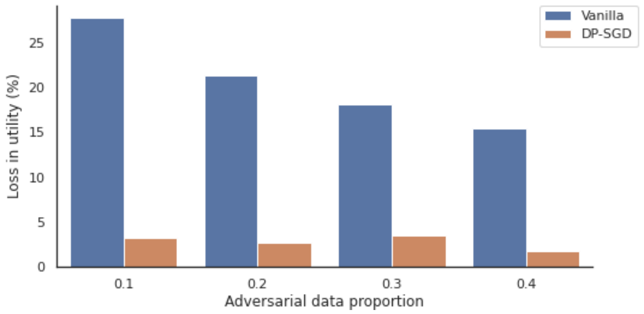


**Fig. 1.** Results for a medium-privacy regime. Accuracy loss under a partially WB attack with adversarial training (generators are the WB models for both, CIFAR-10, ResNet-9). Lower is better.

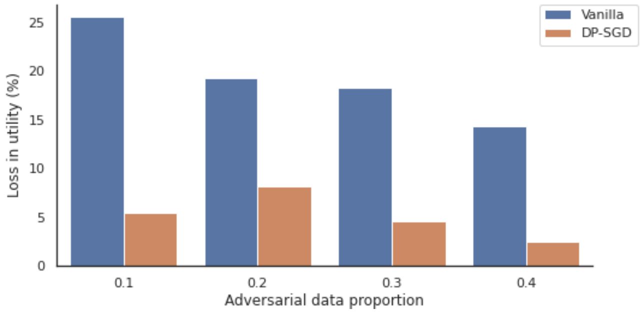


**Fig. 2.** Results for a low-privacy regime. Accuracy loss under a partially WB attack with adversarial training (generators are the WB models for both, CIFAR-10, ResNet-9). Lower is better.

### 1.4 Train-time attacks

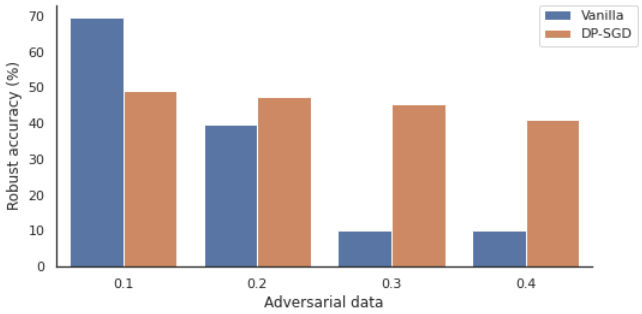


**Fig. 3.** Robust accuracy under a train-time attacker, high-privacy (CIFAR-10, ResNet-18). Higher is better.

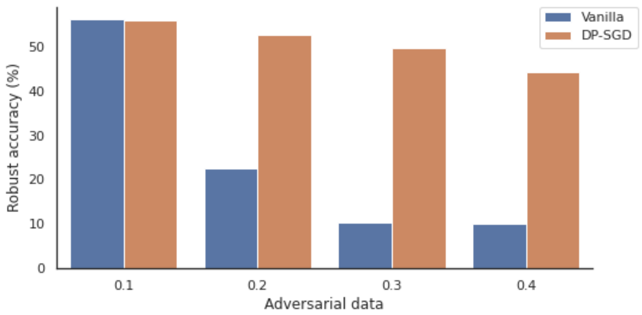


**Fig. 4.** Robust accuracy under a train-time attacker, low-privacy (CIFAR-10, ResNet-9). Higher is better.
